# Supplementary material for: Crowdsourced Fact-Checking at Twitter: How Does the Crowd Compare With Experts?
Source: arXiv:2208.09214 source file (2022-08-19)
Supplement: Supplementary file 1 [file appendix.tex]

\newpage
\appendix
\section{Note and Rating Questions}
Test1

\begin{table}[h]
    \small
    {\begin{tabular}{p{5cm}|p{3cm}}
         \toprule
         \textbf{Input}& \textbf{Possible Output}  \\
         \toprule
        Given current evidence, I believe this tweet is: &
        (1) NOT MISLEADING
        (2) MISINFORMED OR POTENTIALLY MISLEADING
        \\
        \midrule
        If this tweet were widely spread, its message would likely be believed by: & 
        (1) BELIEVABLE BY FEW
        
        (2) BELIEVABLE BY MANY\\
        \midrule
        If many believed this tweet, it might cause:& 
        (1) LITTLE HARM
        (2) CONSIDERABLE HARM\\
        \midrule
        Finding and understanding the correct information would be:&(1) EASY 
        
        (2) CHALLENGING\\
        \midrule
        Is this tweet misleading because it contains a factual error?&True, False\\
        \midrule
        Is this tweet misleading because it contains a digitally altered photo or video?&True, False\\
        \midrule
        Is this tweet misleading because it contains outdated information that may be misleading ?& True, False\\
        \midrule
        Is this tweet misleading because it is a misrepresentation or missing important context?& True, False\\
        \midrule
        Is this tweet misleading because it presents an unverified claim as a fact?& True, False\\
        \midrule
        Is this tweet misleading because it is a joke or satire that might be misinterpreted as a fact?& True, False\\
        \midrule
        Is this tweet misleading for other reasons ?& True, False\\
        \midrule
        Is this tweet not misleading because it expresses a factually correct claim?& True, False\\
        \midrule
        Is this tweet not misleading because it was correct when written, but is out of date now?& True, False\\
        \midrule
        Is this tweet not misleading because it is clearly satirical/joking ?& True, False\\
        \midrule
        Is this tweet not misleading because it expresses a personal opinion?& True, False\\
        \midrule
        Is this tweet not misleading for other reasons ?& True, False\\
        \midrule
        Did you link to sources you believe most people would consider trustworthy?& Yes, No\\
        \bottomrule
    \end{tabular}}
    \caption{Questions to \BW participants when writing a note for a tweet.}
    \label{tab:note_questions}
\end{table}

test2

\begin{table}[h]
    \small
{\begin{tabular}{p{5.5cm}|p{2.1cm}}
         \toprule
         \textbf{Input}& \textbf{Possible Output}  \\
         \toprule
          Do you agree with the note's conclusion?&Yes,No\\
          \midrule
          Is this note helpful?& (1) NOT HELPFUL
          
          (2) SOMEWHAT HELPFUL 
          
          (3) HELPFUL \\
          \midrule
          Is this note helpful because it was clear and/or well-written?& Yes,No\\
          \midrule
          Is this note helpful because it cites high-quality sources?& Yes,No\\
          \midrule
          Is this note helpful because it directly addresses the Tweet’s claim?& Yes,No\\
          \midrule
          Is this note helpful because it provides a neutral or unbiased language?& Yes,No\\
          \midrule
          Is this note helpful for other reasons ?& Yes,No\\
          \midrule
          Is this note unhelpful because it contains incorrect information” ?& Yes,No\\
          \midrule
          Is this note unhelpful because there are sources missing or unreliable?& Yes,No\\
          \midrule
          Is this note unhelpful because it misses key points or irrelevant?& Yes,No\\
          \midrule
          Is this note unhelpful because it is hard to understand?& Yes,No\\
          \midrule
          Is this note unhelpful because it contains an argumentative or biased language?& Yes,No\\
          \midrule
          Is this note unhelpful because it contains spam, harassment, or abuse?& Yes,No\\
          \midrule
          Is this note unhelpful because the sources do not support note?& Yes,No\\
          \midrule
          Is this note unhelpful because it is an opinion or speculation?& Yes,No\\
          \midrule
          Is this note unhelpful because it is not needed on this Tweet?& Yes,No\\
          \midrule
          Is this note unhelpful for other reasons ?& Yes,No\\
         \bottomrule
    \end{tabular}}
    \caption{Questions to \BW participant when rating a note.} \label{tab:rating_questions}
\end{table}
